# Supplementary material for: MeLPUF: Memory-in-Logic PUF Structures for Low-Overhead IC Authentication
Source: arXiv:2012.03162 source file (2023-03-29)
Supplement: Supplementary file 1 [file appendix.tex]

\appendices
\section{Proof of the First Zonklar Equation}
Appendix one text goes here.

% you can choose not to have a title for an appendix
% if you want by leaving the argument blank
\section{}
Appendix two text goes here.

% use section* for acknowledgment
\section*{Acknowledgment}

The authors would like to thank...
